# Supplementary material for: Discrete Wasserstein Flows for One-Step Generative Modeling
Source: arXiv:2610.01355 source file (2026-10-01)
Supplement: Supplementary file 1 [file appendix_kernel.tex]

% Body-only appendix. Requires appendix_preamble.tex in the document preamble.
% Designed for a one-column supplement. No external bibliography keys are used.
\section{Kernel-regularized comparison in discrete Wasserstein drifting}
\label{app:kdd}

\subsection{Purpose and minimal change to the existing implementation}
\label{sec:kdd-scope}

The existing construction transports a model law $q$ toward a target law $p$
by the discrete Wasserstein gradient flow of $\kddKL(q\|p)$. Its transport
kernel $K$ determines where mass can move. It does not, by itself, provide a
sample-based estimate of the logarithmic discrepancy $\log(q/p)$. On a large
finite space, empirical laws are sparse, so an unsmoothed empirical log-ratio
is typically undefined. The purpose of the additional kernel is to regularize
this \emph{comparison}, not to introduce transport or repulsion that was
previously absent.

We keep the transport geometry fixed and choose a smoothing channel
$S_\tau$. The primary proposal is
\begin{equation}
  \boxed{\quad
  \mathcal F_{\tau,p}(q)
    :=\kddKL(qS_\tau\|pS_\tau),
  \qquad
  U_{\tau,p,q}
    :=S_\tau\log\frac{qS_\tau}{pS_\tau}.
  \quad}
  \label{eq:kdd-summary}
\end{equation}
The second expression is a scalar function on states; the operator conventions
are defined below. In the existing current, replace the potential
$\ell_{p,q}=\log(q/p)$ by $U_{\tau,p,q}$. Leave the mobility and the actual law
being transported unchanged. Thus
\begin{equation}
 \boxed{\quad
 J_{\tau,p,q}(x,y)
 =\pi(x)K(x,y)m\!\left(\frac{q(x)}{\pi(x)},\frac{q(y)}{\pi(y)}\right)
   \bigl(U_{\tau,p,q}(x)-U_{\tau,p,q}(y)\bigr).
 \quad}
 \label{eq:kdd-summary-current}
\end{equation}
The outer $S_\tau$ in \eqref{eq:kdd-summary} is required by the chain rule.
It is not an optional second denoising step. No smoothing operator is applied
to generated samples at inference time.

For an initial implementation, use exact $p$ and exact model marginal $q$ on
the existing enumerable torus. Validate the new field before adding either
sample-based potential estimation or neural fitting. This preserves the
manuscript's separation of transport, estimation, and amortization errors.

\subsection{Notation, orientations, and the two kernels}
\label{sec:kdd-notation}

Let $\kddX=\{1,\ldots,N\}$. A probability law is a row vector
$q\in\kddR^{1\times N}$, with $q(x)\geq0$ and $\sum_xq(x)=1$.
Write $\mathcal P(\kddX)$ for the probability simplex and
$\mathcal P_+(\kddX)$ for its strictly positive interior. The reference law
$\pi$ is strictly positive. Relative densities are scalar functions
\begin{equation}
 \rho_q(x)=q(x)/\pi(x).
 \label{eq:kdd-density}
\end{equation}
We retain an irreducible row-stochastic kernel $K$ satisfying detailed balance,
\begin{equation}
 \pi(x)K(x,y)=\pi(y)K(y,x).
 \label{eq:kdd-reversibility}
\end{equation}
The logarithmic mean and existing edge factor are
\begin{align}
 m(a,b)&=\int_0^1 a^s b^{1-s}\,ds
 =\begin{cases}
 (a-b)/(\log a-\log b),&a\ne b,\\
 a,&a=b,
 \end{cases}
 \qquad a,b>0,
 \label{eq:kdd-logmean}\\
 L(r)&=m(1,e^r)
 =\begin{cases}(e^r-1)/r,&r\ne0,\\1,&r=0.\end{cases}
 \label{eq:kdd-L}
\end{align}
For $q>0$, define the symmetric transport weight
\begin{equation}
 w_q(x,y)=\pi(x)K(x,y)m(\rho_q(x),\rho_q(y)).
 \label{eq:kdd-weight}
\end{equation}
All sums over $x,y$ below are over directed pairs. If an implementation stores
one copy of each unordered edge, the factor $1/2$ in quadratic edge sums must
be removed.

\paragraph{Forward action on masses versus action on functions.}
For a row-stochastic smoothing matrix $S$, define
\begin{equation}
 (qS)(y)=\sum_xq(x)S(x,y),
 \qquad
 (Sf)(x)=\sum_yS(x,y)f(y).
 \label{eq:kdd-actions}
\end{equation}
These actions satisfy the duality identity
\begin{equation}
 \sum_y(hS)(y)f(y)=\sum_xh(x)(Sf)(x).
 \label{eq:kdd-duality}
\end{equation}
Consequently, with one-dimensional numerical arrays and $S[x,y]$ storing
transition probability from $x$ to $y$,
\begin{lstlisting}[style=kddpython]
q_smoothed = q @ S
p_smoothed = p @ S
ell = log(q_smoothed) - log(p_smoothed)
U = S @ ell                 # NOT ell @ S on a nonsymmetric chain
\end{lstlisting}
For batched function rows $F$, the pullback is $F S^\top$. If mass vectors
are stored as columns instead, forward smoothing is $S^\top q$ and the
potential is $S\log[(S^\top q)/(S^\top p)]$. Uniform-reference torus tests
alone cannot detect an accidental transpose, because $S$ is symmetric there.

\paragraph{Different roles.}
$K$ controls admissible transport edges and mobility. $S$ controls which
states contribute to each distributional comparison. These roles remain
distinct even when $S$ is constructed from $K$. In particular, rates are
supported on the edges of $K$, not on all the generally dense entries of $S$.

\subsection{A canonical smoothing channel}
\label{sec:kdd-kernel}

Take
\begin{equation}
 H:=I-K,\qquad S_\tau:=e^{-\tau H}=e^{\tau(K-I)},\qquad \tau>0.
 \label{eq:kdd-heat}
\end{equation}
Thus $S_\tau$ is the heat semigroup associated with the existing transport
kernel. All population results below also apply to a fixed strictly positive,
invertible Markov matrix $S$; the heat choice supplies additional spectral
and computational structure.

\begin{kddproposition}[Heat-channel properties]
\label{prop:kdd-heat}
For every finite $\tau>0$, $S_\tau$ is row-stochastic, strictly positive,
invertible, and reversible with invariant law $\pi$. Moreover,
\begin{equation}
 \kappa_\tau(x,y):=\frac{S_\tau(x,y)}{\pi(y)}
 \label{eq:kdd-kappa}
\end{equation}
is a symmetric positive-definite kernel, and
\begin{equation}
 \frac{(qS_\tau)(x)}{\pi(x)}
   =\kddE_{Y\sim q}[\kappa_\tau(x,Y)]
   =(S_\tau\rho_q)(x).
 \label{eq:kdd-kde-density}
\end{equation}
\end{kddproposition}
\begin{proof}
The power series
\begin{equation}
 S_\tau=e^{-\tau}\sum_{r=0}^{\infty}\frac{\tau^r}{r!}K^r
 \label{eq:kdd-poisson}
\end{equation}
is a convex combination of stochastic matrices. Irreducibility implies that,
for each $x,y$, there is some $r\geq0$ with $K^r(x,y)>0$. The corresponding
coefficient in \eqref{eq:kdd-poisson} is positive, proving strict positivity.
Detailed balance is preserved by powers and limits, giving reversibility and
invariance. Matrix exponentials are invertible, with inverse
$e^{\tau H}$; this inverse need not be stochastic and is never needed in the
algorithm.

For positive definiteness, let $D_\pi=\kdddiag(\pi)$ and
$B=D_\pi^{1/2}S_\tau D_\pi^{-1/2}$. Reversibility makes $B$ symmetric.
Since $H$ is self-adjoint in $L^2(\pi)$ with eigenvalues $\lambda_j\geq0$,
$B$ has positive eigenvalues $e^{-\tau\lambda_j}$. The matrix of
$\kappa_\tau$ is $S_\tau D_\pi^{-1}
=D_\pi^{-1/2}BD_\pi^{-1/2}$, hence is symmetric positive definite.
Finally, detailed balance gives
$(qS_\tau)(x)/\pi(x)=\sum_yS_\tau(x,y)q(y)/\pi(y)$, which proves
\eqref{eq:kdd-kde-density}.
\end{proof}

The parameter $\tau$ is a comparison scale, not the transport step size.
Every empirical probability law has a strictly positive image under $S_\tau$,
although its smallest image mass may be extremely small. Positivity in exact
arithmetic is therefore not a uniform guarantee of numerical or statistical
conditioning.

\paragraph{Optional, explicitly declared channel floor.}
A useful numerical variant, separate from the pure heat choice, is
\begin{equation}
 S_{\tau,\varepsilon_s}
  =(1-\varepsilon_s)S_\tau+\varepsilon_s\kddone\pi,
 \qquad 0<\varepsilon_s<1,
 \label{eq:kdd-channel-floor}
\end{equation}
where $(\kddone\pi)(x,y)=\pi(y)$. This matrix remains stochastic,
reversible, and invertible: its constant-mode eigenvalue is $1$ and its other
eigenvalues are $(1-\varepsilon_s)e^{-\tau\lambda_j}>0$.
It satisfies $S_{\tau,\varepsilon_s}(x,y)\geq\varepsilon_s\pi(y)$.
Using this matrix in \emph{both} actions in \eqref{eq:kdd-summary} defines a
precise alternative energy with the same population minimizer. It is not
clipping, and it is not a lower bound on the unsmoothed model masses $q(x)$.
Set $\varepsilon_s=0$ for the primary experiment.

\subsection{Smoothed KL and its exact first variation}
\label{sec:kdd-energy}

Fix a smoothing channel $S=S_\tau$. For $p,q\in\mathcal P(\kddX)$ set
\begin{equation}
 q_\tau=qS,\qquad p_\tau=pS,\qquad
 \mathcal F_{\tau,p}(q)
 =\sum_yq_\tau(y)\log\frac{q_\tau(y)}{p_\tau(y)}.
 \label{eq:kdd-energy}
\end{equation}
Because $S$ is strictly positive, this energy is finite for every $p,q$ in
the simplex. This statement concerns the energy, not the jump rates, which
will still require $q>0$.

\begin{kddproposition}[First and second variations]
\label{prop:kdd-variation}
For a tangent perturbation $h$ satisfying $\sum_xh(x)=0$,
\begin{align}
 D\mathcal F_{\tau,p}(q)[h]
   &=\sum_x h(x)U_{\tau,p,q}(x),
 &U_{\tau,p,q}&=S\log\frac{qS}{pS},
 \label{eq:kdd-first-variation}\\
 D^2\mathcal F_{\tau,p}(q)[h,h]
   &=\sum_y\frac{(hS)(y)^2}{(qS)(y)}.
 \label{eq:kdd-hessian}
\end{align}
The potential is defined up to an additive constant. In unrestricted
probability coordinates the gradient is $\kddone+U_{\tau,p,q}$.
\end{kddproposition}
\begin{proof}
Since $(q+th)S=qS+t(hS)$, differentiation gives
\begin{align*}
 \left.\frac{d}{dt}\mathcal F_{\tau,p}(q+th)\right|_{t=0}
 &=\sum_y(hS)(y)\left(1+\log\frac{(qS)(y)}{(pS)(y)}\right)\\
 &=\sum_xh(x)\sum_yS(x,y)\log\frac{(qS)(y)}{(pS)(y)}.
\end{align*}
The constant vanishes because $S\kddone=\kddone$ and $\sum_xh(x)=0$.
The last expression is \eqref{eq:kdd-first-variation}.
Differentiating once more gives \eqref{eq:kdd-hessian}. Strict positivity of
$qS$ also gives a smooth extension to a neighborhood of every point of the
closed simplex, so these formulas remain meaningful at its boundary along
admissible directions.
\end{proof}

\begin{kddcorollary}[Identifiability and absence of population smoothing bias]
\label{cor:kdd-identifiability}
If $S$ is invertible, $\mathcal F_{\tau,p}$ is strictly convex and has the
unique minimizer $p$, with minimum value zero.
\end{kddcorollary}
\begin{proof}
For $h\ne0$, invertibility gives $hS\ne0$, so
\eqref{eq:kdd-hessian} is strictly positive. Also,
$\mathcal F_{\tau,p}(q)=0$ if and only if $qS=pS$, which is equivalent
to $q=p$.
\end{proof}

\paragraph{Three modifications that must not be conflated.}
Changing only $K$ changes transport geometry but leaves the original log-ratio
estimation problem. Replacing the original target by $pS$ and minimizing
$\kddKL(q\|pS)$ targets the smoothed law $pS$. In contrast,
$\kddKL(qS\|pS)$ compares smoothed laws but still targets the unsmoothed
law $p$. The last statement does not imply faster optimization or better
finite-sample generalization.

\paragraph{Why the outer operator is necessary.}
Let $\widetilde U=\log(qS/pS)$ and construct a current from differences of
$\widetilde U$ rather than $U=S\widetilde U$. The derivative of the
smoothed energy along that alternative current would be
\begin{equation}
 -\frac12\sum_{x,y}w_q(x,y)
       \bigl(U(x)-U(y)\bigr)
       \bigl(\widetilde U(x)-\widetilde U(y)\bigr).
 \label{eq:kdd-wrong-potential}
\end{equation}
This is not a negative sum of squares. The dissipation proof below does not
apply to this plug-in force. Freezing a teacher with stop-gradient does not
change the functional derivative that must be derived \emph{before} freezing.

\paragraph{Normalization freedom is retained, locality is not.}
Let $\widetilde q=c_q q$ and $\widetilde p=c_p p$ be unnormalized positive
masses, with $c_q,c_p>0$. Then
\begin{equation}
 S\log\frac{\widetilde qS}{\widetilde pS}
  =U+\log(c_q/c_p)\kddone.
 \label{eq:kdd-normalization}
\end{equation}
All edge differences are unchanged. Thus partition functions are unnecessary
for the potential differences. However, evaluating a smoothed mass generally
requires information beyond one transport edge. The extension is
normalization-free but is no longer purely edge-local in its target
information requirements. If the existing implementation exposes only local
target scores, it must additionally provide a smoothing application or a
sample-based approximation to the smoothed target.

\subsection{Maas flow, dissipation, and the scope of stationarity}
\label{sec:kdd-flow}

For $q>0$, define
\begin{align}
 J_{\tau,p,q}(x,y)&=w_q(x,y)\bigl(U_{\tau,p,q}(x)-U_{\tau,p,q}(y)\bigr),
 \label{eq:kdd-current}\\
 v_{\tau,p}(q)(x)&=-\sum_yJ_{\tau,p,q}(x,y),
 &\dot q_t&=v_{\tau,p}(q_t).
 \label{eq:kdd-flow}
\end{align}
This is the discrete Wasserstein gradient flow of
$\mathcal F_{\tau,p}$ with the existing logarithmic-mean geometry.
In the manuscript's continuity-equation convention, its velocity potential
is $\psi=-U$, not $U$.

\begin{kddtheorem}[Dissipation and interior stationary points]
\label{thm:kdd-dissipation}
Let $q_t$ be a differentiable solution of \eqref{eq:kdd-flow} on an interval
where $q_t>0$. Total mass is conserved, and
\begin{align}
 \frac{d}{dt}\mathcal F_{\tau,p}(q_t)
  &=-\mathcal I_{\tau,K}(q_t\mid p),
 \label{eq:kdd-dissipation}\\
 \mathcal I_{\tau,K}(q\mid p)
  &:=\frac12\sum_{x,y}w_q(x,y)
       \bigl(U_{\tau,p,q}(x)-U_{\tau,p,q}(y)\bigr)^2.
 \label{eq:kdd-information}
\end{align}
If $p>0$, then for $q>0$ the following are equivalent:
\begin{equation}
 v_{\tau,p}(q)=0,
 \qquad \mathcal I_{\tau,K}(q\mid p)=0,
 \qquad q=p.
 \label{eq:kdd-stationarity}
\end{equation}
If $p$ has zero entries, the energy still has unique minimizer $p$, but no
interior stationary point exists.
\end{kddtheorem}
\begin{proof}
The weight $w_q$ is symmetric, so $J(x,y)=-J(y,x)$. Summing the current
divergence gives zero total mass change. Using
\eqref{eq:kdd-first-variation} and pairing the two orientations of each edge,
\begin{align*}
 \frac{d}{dt}\mathcal F_{\tau,p}(q_t)
 &=-\sum_{x,y}U(x)w_{q_t}(x,y)(U(x)-U(y))\\
 &=-\frac12\sum_{x,y}w_{q_t}(x,y)(U(x)-U(y))^2.
\end{align*}
At a stationary point the left-hand side is zero. Conversely, zero
dissipation makes each supported edge difference vanish because $q>0$.
Connectedness of the graph gives $U=c\kddone$. Since
$U=S\log(qS/pS)$, invertibility and $S\kddone=\kddone$ yield
$\log(qS/pS)=c\kddone$. Normalization forces $e^c=1$, then $qS=pS$
and $q=p$. At $q=p$, $U=0$ and the current vanishes. If $p$ is on the
boundary, the same argument rules out any stationary $q>0$.
\end{proof}

The theorem establishes dissipation of the \emph{smoothed} energy. It does
not establish that the original $\kddKL(q_t\|p)$ decreases along the
modified flow. It also does not claim global convergence from every starting
law or a uniform convergence rate. Local existence and uniqueness in the
interior follow from smoothness of the vector field there; continuation up
to a boundary or asymptotic convergence requires additional analysis.

\paragraph{Boundary degeneracy remains.}
The continuous extension of the logarithmic mean satisfies $m(a,0)=0$.
For fixed positive $S$, the potential is finite even at a boundary law.
Consequently, any edge incident to a zero-mass endpoint has zero weight under
the continuous extension of \eqref{eq:kdd-weight}. At a point mass, every
edge weight between distinct states is zero, so the extended current is zero
although the energy is generally not minimized. This is a statement about
the extended \emph{current}; the rate formula dividing by $q(x)$ is undefined
at zero-mass states. We therefore do not construct the transported law from
a sparse particle histogram. Use the strictly positive generator marginal,
and do not interpret smoothing the comparison as removing this restriction.

\subsection{Minimal particle rates and frozen probability updates}
\label{sec:kdd-particles}

For $q>0$ and $x\ne y$, define
\begin{equation}
 a_{\tau,p,q}(x,y)=\frac{[J_{\tau,p,q}(x,y)]_+}{q(x)},
 \qquad [r]_+=\max\{r,0\}.
 \label{eq:kdd-rates}
\end{equation}
Set $A(x,y)=a(x,y)$ off the diagonal and
$A(x,x)=-\sum_{y\ne x}a(x,y)$. The quantity
\begin{equation}
 \lambda_q(x):=\sum_{y\ne x}a(x,y)
 \label{eq:kdd-exit}
\end{equation}
is the exit rate. Positive $J(x,y)$ means mass flows from $x$ to $y$; positive
$U(x)-U(y)$ therefore causes a jump from the larger potential to the smaller
potential.

\begin{kddproposition}[Exact realization and edgewise minimality]
\label{prop:kdd-particles}
$A$ is a continuous-time Markov generator and
\begin{equation}
 (qA)(x)=-\sum_yJ(x,y)=v_{\tau,p}(q)(x).
 \label{eq:kdd-qA}
\end{equation}
Any nonnegative rates $b(x,y),b(y,x)$ with the same signed traffic satisfy,
for a unique $r_{x,y}\geq0$,
\begin{align}
 q(x)b(x,y)&=[J(x,y)]_++r_{x,y},\\
 q(y)b(y,x)&=[-J(x,y)]_++r_{x,y}.
\end{align}
Their total edge traffic is $|J(x,y)|+2r_{x,y}$. Thus
\eqref{eq:kdd-rates} is the unique realization minimizing probability traffic
on each edge. At $q=p>0$, all its rates vanish.
\end{kddproposition}
\begin{proof}
Nonnegative off-diagonal entries and zero row sums make $A$ a Markov
generator. At state $x$,
\begin{align*}
 (qA)(x)
 &=\sum_{y\ne x}\bigl(q(y)a(y,x)-q(x)a(x,y)\bigr)\\
 &=\sum_{y\ne x}\bigl([-J(x,y)]_+-[J(x,y)]_+\bigr)
 =-\sum_yJ(x,y).
\end{align*}
For minimality write $u=q(x)b(x,y)$ and $v=q(y)b(y,x)$.
The constraint $u-v=J$ implies
$u=[J]_++\min(u,v)$ and $v=[-J]_++\min(u,v)$.
This identifies the unique nonnegative $r_{x,y}$ and the traffic formula.
At equilibrium $U=0$, hence $J=0$ and the minimal rates are zero.
\end{proof}

Using the homogeneity identity
$m(\rho_q(x),\rho_q(y))=\rho_q(x)L(\delta_q(x,y))$, where
\begin{equation}
 \delta_q(x,y):=\log\rho_q(y)-\log\rho_q(x),
\end{equation}
the implementation-equivalent rate formula is
\begin{equation}
 \boxed{\quad a_{\tau,p,q}(x,y)
  =K(x,y)L(\delta_q(x,y))
    [U_{\tau,p,q}(x)-U_{\tau,p,q}(y)]_+.\quad}
 \label{eq:kdd-rate-logit}
\end{equation}
The density difference in $L$ is that of $q$, not $qS$.

\paragraph{One frozen stay-or-jump transition.}
Freeze $A$ at the current law and define
\begin{equation}
 P_\eta=I+\eta A.
 \label{eq:kdd-P}
\end{equation}
For
\begin{equation}
 \eta\max_x\lambda_q(x)\leq1,
 \label{eq:kdd-cfl}
\end{equation}
$P_\eta$ is stochastic and
\begin{equation}
 qP_\eta=q+\eta v_{\tau,p}(q).
 \label{eq:kdd-euler-exact}
\end{equation}
This is an exact identity for the explicit Euler step, not an exact integration
of the nonlinear flow over time $\eta$. Likewise, $e^{\eta A(q)}$ would
integrate the \emph{frozen linear} generator, not the law-dependent generator
recomputed continuously along the flow.

For a particle currently at $x$, stay with probability $1-\eta\lambda_q(x)$.
Otherwise draw a neighbor $y$ with probability $a(x,y)/\lambda_q(x)$.
When $\lambda_q(x)=0$, stay deterministically. This procedure uses at most
one jump per outer step.

\paragraph{Strict positivity and a shared time step.}
Choose a global safety factor $c_{\rm CFL}\in(0,1)$ and
\begin{equation}
 \eta=\min\left\{\eta_{\max},
              \frac{c_{\rm CFL}}{\max_x\lambda_q(x)}\right\},
 \label{eq:kdd-safe-step}
\end{equation}
with the second term interpreted as $+\infty$ if all rates vanish.
Then $P_\eta(x,x)\geq1-c_{\rm CFL}>0$ and
\begin{equation}
 (qP_\eta)(x)\geq(1-c_{\rm CFL})q(x)>0.
 \label{eq:kdd-interior-step}
\end{equation}
A common scalar $\eta$ is part of the specified Euler step. Independently
clipping each row's rates, using state-dependent step sizes, or normalizing
rows after an inadmissible step changes the prescribed flow.

\subsection{Logit dynamics and the zero-smoothing limit}
\label{sec:kdd-logits}

Retain the manuscript's log-density chart
\begin{equation}
 q_g(x)=\frac{\pi(x)e^{g(x)}}{Z_\pi(g)},
 \qquad Z_\pi(g)=\sum_z\pi(z)e^{g(z)}.
 \label{eq:kdd-chart}
\end{equation}
For nonuniform $\pi$, an ordinary softmax over $g$ alone is not this chart:
it is the softmax over $g+\log\pi$.
Define
\begin{equation}
 \Delta_{\tau,g}(x)
  :=\sum_yK(x,y)L(g(y)-g(x))
           \bigl(U_{\tau,p,q_g}(y)-U_{\tau,p,q_g}(x)\bigr).
 \label{eq:kdd-delta}
\end{equation}

\begin{kddproposition}[Chart representation and local consistency]
\label{prop:kdd-chart}
For every $g$,
\begin{equation}
 v_{\tau,p}(q_g)=q_g\odot\Delta_{\tau,g},
 \qquad \sum_xq_g(x)\Delta_{\tau,g}(x)=0.
 \label{eq:kdd-centering}
\end{equation}
The law $q_{g_t}$ solves \eqref{eq:kdd-flow} if and only if
$\dot g_t=\Delta_{\tau,g_t}+c_t\kddone$ for some scalar gauge $c_t$.
For fixed $g$, as $\eta\to0$,
\begin{align}
 q_{g+\eta\Delta_{\tau,g}}
   &=q_g+\eta q_g\odot\Delta_{\tau,g}+O(\eta^2),
 \label{eq:kdd-chart-euler}\\
 \mathcal F_{\tau,p}(q_{g+\eta\Delta_{\tau,g}})
   &=\mathcal F_{\tau,p}(q_g)
       -\eta\mathcal I_{\tau,K}(q_g\mid p)+O(\eta^2).
 \label{eq:kdd-chart-descent}
\end{align}
If \eqref{eq:kdd-cfl} holds, the probability represented by the updated logits
and $q_gP_\eta$ differ by $O(\eta^2)$.
\end{kddproposition}
\begin{proof}
Divide the current divergence by $q_g(x)$ and use logarithmic-mean
homogeneity to obtain \eqref{eq:kdd-delta}. Summing the divergence proves
centering. The differential of the chart is
\begin{equation}
 Dq_g[h](x)=q_g(x)\left(h(x)-\sum_zq_g(z)h(z)\right).
 \label{eq:kdd-chart-differential}
\end{equation}
Comparison with \eqref{eq:kdd-centering} proves the gauge characterization.
Taylor expansion and centering give \eqref{eq:kdd-chart-euler}.
Applying the first variation and the dissipation identity gives
\eqref{eq:kdd-chart-descent}. Finally, \eqref{eq:kdd-euler-exact} has
exactly the same first-order term as \eqref{eq:kdd-chart-euler}.
\end{proof}

A unit-learning-rate gradient step on the tabular regression
\begin{equation}
 \mathcal L_{\rm logit}(g;\bar g)
 =\frac12\sum_x\left(g(x)-\kddsg[\bar g(x)+\eta\Delta_{\tau,\bar g}(x)]\right)^2
 \label{eq:kdd-logit-loss}
\end{equation}
implements this chart update when $g$ itself is the parameter vector and the
step starts at $\bar g$. This exact one-gradient-step property does not
extend to a shared neural parametrization. Directly minimizing
$\mathcal F_{\tau,p}(q_\theta)$ with an ordinary Euclidean parameter optimizer
is also not, in general, the Maas flow specified here.

For fixed $p,q>0$, $S_\tau\to I$ as $\tau\downarrow0$, hence
\begin{equation}
 U_{\tau,p,q}\longrightarrow\log(q/p).
 \label{eq:kdd-zero-limit}
\end{equation}
If $s_p(x,y)=\log\rho_p(y)-\log\rho_p(x)$, then
\begin{equation}
 \Delta_{\tau,g}(x)\longrightarrow
 \sum_yK(x,y)L(g(y)-g(x))\bigl(g(y)-g(x)-s_p(x,y)\bigr).
 \label{eq:kdd-original-recovery}
\end{equation}
Thus the original drift is recovered. The limit requires fixed positive laws;
it is not uniform over sparse empirical distributions. For a declared channel
floor \eqref{eq:kdd-channel-floor}, recovering the original method additionally
requires $\varepsilon_s\to0$.

\subsection{Frozen conditional teachers and neural fitting}
\label{sec:kdd-amortization}

Let $R_{k,z}=G_{\theta_k}(\cdot\mid z)$ and
$q_k=\kddE_{z\sim\nu}[R_{k,z}]$. Build one field and one transition matrix
from this \emph{marginal}, then define
\begin{equation}
 T_{k,z}=\kddsg[R_{k,z}P_{\eta_k}(q_k)].
 \label{eq:kdd-teachers}
\end{equation}
The same frozen transition is used for every latent. Neither the smoothing
scale nor the rates are recomputed inside the inner optimization loop.
For a finite fixed latent bank $z_1,\ldots,z_B$, replace the expectation by
$B^{-1}\sum_i$. This defines an exact finite-prior marginal, rather than an
exact Gaussian-prior marginal.

\begin{kddproposition}[Teacher marginal and fitting error]
\label{prop:kdd-teachers}
For any frozen stochastic matrix $P$,
\begin{equation}
 \kddE_z[T_{k,z}]=q_kP.
 \label{eq:kdd-teacher-marginal}
\end{equation}
If $\bar q_{k+1}=\kddE_z[G_{\theta_{k+1}}(\cdot\mid z)]$, then
\begin{equation}
 \kddTV(\bar q_{k+1},q_kP)
  \leq\kddE_z\kddTV\bigl(G_{\theta_{k+1}}(\cdot\mid z),T_{k,z}\bigr).
 \label{eq:kdd-fitting-TV}
\end{equation}
\end{kddproposition}
\begin{proof}
Linearity of multiplication by a fixed matrix gives
$\kddE_z[R_{k,z}P]=(\kddE_zR_{k,z})P$.
For total variation, write each coordinate of the marginal difference as an
expectation and use $|\kddE X|\leq\kddE|X|$, then sum and divide by two.
\end{proof}

Fit the teachers with the same conditional cross-entropy used in the
manuscript,
\begin{equation}
 \mathcal L_k(\theta)
 =-\kddE_z\sum_x T_{k,z}(x)\log G_\theta(x\mid z).
 \label{eq:kdd-CE}
\end{equation}
The teachers, old conditionals, marginal, smoothed laws, potential, mobility,
rates, and selected step size are all detached from the inner computation
graph. Gradients are taken only through the current predictions
$G_\theta(x\mid z)$. Exact fitting yields the probability Euler step;
finite fitting need not preserve energy descent at every outer iteration.

When enumerating each conditional is impractical but its categorical law can
be sampled and scored, draw $X\sim R_{k,z}$, then
$Y\sim P_{\eta_k}(X,\cdot)$, and train on $-\log G_\theta(Y\mid z)$.
Conditional on the frozen teacher construction, its expectation is
\eqref{eq:kdd-CE}. Keep the latent label $z$ attached to its transported
sample. Resampling or dropping that association changes the conditional
learning problem.

\begin{algorithm}[tbp]
\caption{Exact finite-bank smoothed-KL drifting: one outer iteration}
\label{alg:kdd-exact}
\begin{algorithmic}[1]
\Require Fixed bank $z_1,\ldots,z_B$; target $p$; geometry $K,\pi$;
channels $S_r$ and weights $\alpha_r>0$; $\eta_{\max}$; $c_{\rm CFL}\in(0,1)$
\State Cache $p_r\gets pS_r$ for all scales while $p,S_r$ are unchanged
\State Evaluate $R_i\gets G_{\bar\theta}(\cdot\mid z_i)$ without gradients
\State $q\gets B^{-1}\sum_iR_i$; verify $q(x)>0$ for every state
\State $U\gets0$, $F\gets0$
\For{each scale $r$}
  \State $q_r\gets qS_r$, $\ell_r\gets\log q_r-\log p_r$
  \State $U\gets U+\alpha_rS_r\ell_r$;
         $F\gets F+\alpha_r\sum_yq_r(y)\ell_r(y)$
\EndFor
\State Optionally center $U\gets U-(\sum_xq(x)U(x))\kddone$
\State Build $w_q(x,y)$ from the unsmoothed marginal $q$
\State $J(x,y)\gets w_q(x,y)(U(x)-U(y))$ on transport edges
\State $a(x,y)\gets[J(x,y)]_+/q(x)$; $\lambda(x)\gets\sum_{y\ne x}a(x,y)$
\State Select one global $\eta$ by \eqref{eq:kdd-safe-step}
\State Optionally backtrack $\eta$ against the fixed smoothed energy
\State Construct every $T_i\gets R_i(I+\eta A)$ using the sparse update
\State Freeze $\{T_i\}_{i=1}^B$
\State Starting at $\bar\theta$, take the prescribed inner optimizer steps on
$-B^{-1}\sum_{i,x}T_i(x)\log G_\theta(x\mid z_i)$
\State Log transport diagnostics separately from fitting diagnostics
\Ensure Updated generator parameters; inference remains one-step
\end{algorithmic}
\end{algorithm}

\subsection{Sample-based potentials and what they do not estimate}
\label{sec:kdd-estimation}

The potential can be estimated without assigning a positive empirical mass
to every state. This does not remove the separate need for the actual
unsmoothed marginal or its local ratios in the mobility.

\subsubsection{Inner kernel averages}

Let $Y_1,\ldots,Y_{M_p}\sim p$ and $X_1,\ldots,X_{M_q}\sim q$ be independent
i.i.d. sample sets. For fixed $S=S_\tau$ define
\begin{align}
 \widehat p_\tau(y)&=\frac1{M_p}\sum_{i=1}^{M_p}S(Y_i,y),
 &\widehat q_\tau(y)&=\frac1{M_q}\sum_{j=1}^{M_q}S(X_j,y),
 \label{eq:kdd-empirical-smoothed}\\
 \widehat\ell_\tau(y)&=\log\widehat q_\tau(y)-\log\widehat p_\tau(y),
 &\widehat U_\tau(x)&=(S\widehat\ell_\tau)(x).
 \label{eq:kdd-estimated-potential}
\end{align}
The smoothed mass estimates are unbiased and strictly positive; their
log-ratio and the resulting potential are generally biased at finite sample
size. When all states can be enumerated, these expressions are equivalent to
forming histograms $\widehat p,\widehat q$ and applying the forward channel.
The histograms may have zeros because they are used only for the comparison.
Build the transport weights from the positive model law $q$, not from
$\widehat q$.

A useful first stochastic experiment estimates only the target:
\begin{equation}
 \widehat U_\tau=S\log\frac{qS}{\widehat pS}.
 \label{eq:kdd-target-only-estimation}
\end{equation}
This retains exact model smoothing and exact model mobility. For a fixed
empirical target $\widehat p$, it is the exact potential of
$\kddKL(qS\|\widehat pS)$. Estimating both smoothed laws introduces a
second and distinct source of force error.

\begin{kddproposition}[A finite-state potential-error bound]
\label{prop:kdd-estimation-bound}
Let $a_\tau=\min_{x,y}S(x,y)>0$ and $b_\tau=\max_{x,y}S(x,y)$.
With probability at least $1-\delta$,
\begin{equation}
 \|\widehat U_\tau-U_\tau\|_\infty
 \leq\frac{b_\tau-a_\tau}{a_\tau}
       \sqrt{\frac{\log(4N/\delta)}{2}}
       \left(\frac1{\sqrt{M_q}}+\frac1{\sqrt{M_p}}\right).
 \label{eq:kdd-estimation-bound}
\end{equation}
\end{kddproposition}
\begin{proof}
Every empirical and population smoothed mass lies in $[a_\tau,b_\tau]$.
For an average of $M$ independent variables in this interval, the bounded-
variable exponential concentration bound gives
\begin{equation}
 \Pr(|\widehat r_\tau(y)-r_\tau(y)|\geq t)
 \leq 2\exp\!\left(-\frac{2Mt^2}{(b_\tau-a_\tau)^2}\right).
\end{equation}
If $a_\tau=b_\tau$, all estimates are constant and the desired conclusion is
immediate. Otherwise, a union bound over $N$ states and both sample sets
bounds their sup-norm errors by
$(b_\tau-a_\tau)\sqrt{\log(4N/\delta)/(2M_q)}$ and the corresponding
$M_p$ expression. Since $\log$ is $1/a_\tau$-Lipschitz on this interval,
\begin{equation}
 \|\widehat\ell_\tau-\ell_\tau\|_\infty
 \leq a_\tau^{-1}\bigl(
    \|\widehat q_\tau-q_\tau\|_\infty
   +\|\widehat p_\tau-p_\tau\|_\infty\bigr).
\end{equation}
Finally, a stochastic matrix is a contraction in the function sup norm:
$\|Sf\|_\infty\leq\|f\|_\infty$. Combining these inequalities proves
\eqref{eq:kdd-estimation-bound}.
\end{proof}

This worst-case bound becomes uninformative when $a_\tau$ is extremely
small. In high-dimensional product spaces, positivity alone is not a cure
for poor sample efficiency. No favorable dimension-free estimation claim is
made here.

\subsubsection{Outer Monte Carlo and shared state potentials}

If applying $S$ to a whole function is expensive but corruption sampling is
available, conditionally on $\widehat\ell_\tau$ draw
$Z_1^{(x)},\ldots,Z_{M_U}^{(x)}\sim S(x,\cdot)$ and use
\begin{equation}
 \widehat U_{\tau,M_U}(x)
   =\frac1{M_U}\sum_{r=1}^{M_U}\widehat\ell_\tau(Z_r^{(x)}).
 \label{eq:kdd-outer-MC}
\end{equation}
This is conditionally unbiased for $S\widehat\ell_\tau(x)$, not generally
unbiased for the population $U_\tau(x)$. Let
$B_\tau=\log(b_\tau/a_\tau)$. Because
$|\widehat\ell_\tau(y)|\leq B_\tau$, conditional concentration and a
union bound imply, with probability at least $1-\delta_U$,
\begin{equation}
 \|\widehat U_{\tau,M_U}-\widehat U_\tau\|_\infty
   \leq B_\tau\sqrt{\frac{2\log(2N/\delta_U)}{M_U}}.
 \label{eq:kdd-outer-bound}
\end{equation}
Use this with a separate failure budget from
Proposition~\ref{prop:kdd-estimation-bound}. Only the evaluated states need
be included in a conditional union bound over a fixed query set.

Cache one estimated scalar potential per queried state within each outer
step and reuse it on every incident edge. Then the realized current is
antisymmetric for that realized function. Independently resampling different
values for the same endpoint on opposite orientations need not preserve
antisymmetry. Cache the inner sample sets as well. Efficient evaluation of
$S(x,y)$ and sampling from $S(x,\cdot)$ are additional algorithmic
requirements; these operations need not be cheap on an arbitrary state space.

\subsubsection{Error in the potential versus error in the mobility}

Suppose the actual transported law and its mobility are exact, but the
potential used by the update is $\widehat U=U+e$. Define the edge inner product
\begin{equation}
 \langle f,g\rangle_{q,K}
 =\frac12\sum_{x,y}w_q(x,y)
       (f(x)-f(y))(g(x)-g(y)),
 \qquad \|f\|_{q,K}^2=\langle f,f\rangle_{q,K}.
 \label{eq:kdd-edge-norm}
\end{equation}
It is a seminorm because constants have zero norm.

\begin{kddproposition}[Perturbed dissipation and one-step force error]
\label{prop:kdd-perturbation}
The current built from $\widehat U$ satisfies
\begin{equation}
 \frac{d}{dt}\mathcal F_{\tau,p}(q_t)
  =-\|U\|_{q,K}^2-\langle U,e\rangle_{q,K}
  \leq-\frac12\|U\|_{q,K}^2+\frac12\|e\|_{q,K}^2.
 \label{eq:kdd-perturbed-dissipation}
\end{equation}
On every directed edge,
\begin{align}
 |\widehat J(x,y)-J(x,y)|
    &=w_q(x,y)|e(x)-e(y)|,
 \label{eq:kdd-J-error}\\
 |\widehat a(x,y)-a(x,y)|
    &\leq\frac{w_q(x,y)}{q(x)}|e(x)-e(y)|.
 \label{eq:kdd-rate-error}
\end{align}
Let $\mathcal E_u$ contain one copy of every unordered transport edge.
For a common step size admissible for both frozen generators,
\begin{equation}
 \kddTV(q\widehat P_\eta,qP_\eta)
   \leq\eta\sum_{\{x,y\}\in\mathcal E_u}
                   w_q(x,y)|e(x)-e(y)|.
 \label{eq:kdd-step-error}
\end{equation}
\end{kddproposition}
\begin{proof}
Differentiate the true energy along the estimated current and pair edges.
The result is $-\langle U,U+e\rangle_{q,K}$. Cauchy--Schwarz and
$ab\leq(a^2+b^2)/2$ give \eqref{eq:kdd-perturbed-dissipation}.
Equation~\eqref{eq:kdd-J-error} follows by subtraction; the scalar positive
part is $1$-Lipschitz, proving \eqref{eq:kdd-rate-error}. Finally, the
probability Euler difference is the divergence of $\eta(\widehat J-J)$.
Its $\ell^1$ norm is at most the sum of the absolute directed currents,
which equals twice the unordered-edge sum. Divide by two for total variation.
\end{proof}

Combining \eqref{eq:kdd-fitting-TV} and \eqref{eq:kdd-step-error} gives the
one-step separation
\begin{align}
 \kddTV(\bar q_{k+1},qP_\eta)
 \leq{}&\kddE_z\kddTV\bigl(G_{\theta_{k+1}}(\cdot\mid z),
                               R_{k,z}\widehat P_\eta\bigr)\nonumber\\
 &+\eta\sum_{\{x,y\}\in\mathcal E_u}w_q(x,y)|e(x)-e(y)|.
 \label{eq:kdd-combined-error}
\end{align}
This separates local fitting error from potential-estimation error at a common
starting law and common step size. It is not a global rollout error bound and
excludes numerical error, different adaptive step choices, and mobility error.

The kernel does not estimate the unsmoothed ratio
$\rho_q(y)/\rho_q(x)$ appearing in \eqref{eq:kdd-rate-logit}. For the
initial implementation, compute that ratio from the exact positive marginal.
At scale, a separate marginal-ratio estimator is necessary. Replacing the
mobility by one built from smoothed or independently estimated edge ratios
changes the specified method. In particular, arbitrary independently fitted
oriented ratios need not define a consistent node law or symmetric edge
weight. The guarantees above do not cover that substitution.

\paragraph{Population equilibrium versus finite-data behavior.}
At the population equality $q=p$, exact potentials and minimal rates vanish.
Independent finite sample sets can still produce a nonzero estimated field,
and the positive-part operation can introduce additional finite-sample rate
bias. Conversely, for a fixed dataset $\widehat p$, invertibility of $S$
implies that $\kddKL(qS\|\widehat pS)$ is uniquely minimized by
$q=\widehat p$. A smoothing kernel regularizes the comparison signal; it
does not, by itself, turn an empirical objective into a population
generalization guarantee. With new target batches at each iteration, there is
also no single fixed empirical energy whose pathwise decrease is guaranteed.

\begin{algorithm}[tbp]
\caption{Sample-based potential with exact positive model mobility}
\label{alg:kdd-estimated}
\begin{algorithmic}[1]
\Require Positive model marginal $q$; target and model comparison samples;
channel $S$; queried states and their transport neighbors
\State Freeze the comparison sample sets for this outer iteration
\State Form $\widehat p_\tau(y)$ and $\widehat q_\tau(y)$ by
\eqref{eq:kdd-empirical-smoothed} at required comparison locations
\State $\widehat\ell_\tau(y)\gets\log\widehat q_\tau(y)-\log\widehat p_\tau(y)$
\State Compute $\widehat U=S\widehat\ell_\tau$ exactly, or estimate by
\eqref{eq:kdd-outer-MC}
\State Cache one value of $\widehat U(x)$ per queried state
\State Build $w_q$ from the actual positive model marginal, not the sample histogram
\State $\widehat J(x,y)\gets w_q(x,y)(\widehat U(x)-\widehat U(y))$
\State Set the reverse current to its exact negative
\State $\widehat a(x,y)\gets[\widehat J(x,y)]_+/q(x)$
\State Select a valid global step or a separately justified scalable alternative
\State Construct and freeze teachers using the resulting common transition
\State Fit as in Algorithm~\ref{alg:kdd-exact}
\Ensure A stochastic teacher update; exact population dissipation is not asserted
\end{algorithmic}
\end{algorithm}

\subsection{Bandwidth, multiscale comparison, and annealing}
\label{sec:kdd-scales}

\subsubsection{A spectral calculation at the reference equilibrium}

The bandwidth trades statistical averaging against force resolution. This
can be calculated explicitly when $p=\pi$. Since $H=I-K$ is self-adjoint
in $L^2(\pi)$, take an orthonormal eigenbasis with
$H\varphi_j=\lambda_j\varphi_j$, $\lambda_0=0$, and
$\lambda_j>0$ on nonconstant modes. Write a small perturbation as
\begin{equation}
 \rho_q=1+\epsilon h,\qquad
 \langle h,1\rangle_\pi=0,
 \qquad \langle f,g\rangle_\pi=\sum_x\pi(x)f(x)g(x).
\end{equation}
Reversibility gives $\rho_{qS_\tau}=S_\tau\rho_q$. Therefore
\begin{align}
 U_{\tau,\pi,q}
   &=S_\tau\log(1+\epsilon S_\tau h)
     =\epsilon S_\tau^2h+O(\epsilon^2),
 \label{eq:kdd-linear-U}\\
 \mathcal F_{\tau,\pi}(q)
   &=\frac{\epsilon^2}{2}\|S_\tau h\|_{L^2(\pi)}^2
       +O(\epsilon^3).
 \label{eq:kdd-linear-energy}
\end{align}
At equilibrium $m(1,1)=1$. In relative-density coordinates, linearization
of \eqref{eq:kdd-flow} consequently gives
\begin{equation}
 \boxed{\dot h=-HS_\tau^2h.}
 \label{eq:kdd-linear-flow}
\end{equation}
The coefficient $h_j=\langle h,\varphi_j\rangle_\pi$ satisfies
\begin{equation}
 \boxed{\dot h_j=-\lambda_j e^{-2\tau\lambda_j}h_j.}
 \label{eq:kdd-mode-rate}
\end{equation}
At a fixed normalization of flow time, smoothing slows every nonconstant
oracle mode in this calculation. Its possible benefit is a better estimated
force, not universal acceleration of the exact flow. Finite-$\tau$
invertibility means identifiability is retained; it does not prevent severe
ill-conditioning. As $\tau\to\infty$, $S_\tau\to\kddone\pi$ and all
comparisons become uninformative.

\subsubsection{Fixed multiscale energy}

For fixed scales $\tau_1,\ldots,\tau_R>0$ and weights $\alpha_r>0$, define
\begin{align}
 \mathcal F_{\boldsymbol\tau,p}(q)
   &=\sum_{r=1}^R\alpha_r
            \kddKL(qS_{\tau_r}\|pS_{\tau_r}),
 \label{eq:kdd-multiscale-energy}\\
 U_{\boldsymbol\tau,p,q}
   &=\sum_{r=1}^R\alpha_r S_{\tau_r}
                   \log\frac{qS_{\tau_r}}{pS_{\tau_r}}.
 \label{eq:kdd-multiscale-U}
\end{align}
Weights summing to one provide a convenient common normalization for
comparisons across the number of scales, but normalization is not needed for
the proofs. With this potential, all current, dissipation, stationary-point,
particle, and teacher results above continue to hold. Strict convexity follows
by summing the positive Hessian quadratic forms. The dissipation is the
squared edge seminorm of the \emph{combined} potential, not the sum of
scale-wise dissipations. At $p=\pi$, the linearized mode rate is
\begin{equation}
 \lambda_j\sum_{r=1}^R\alpha_r e^{-2\tau_r\lambda_j}.
 \label{eq:kdd-multiscale-spectrum}
\end{equation}
A small scale retains less-attenuated fine-resolution forces, while larger
scales average more broadly.

Because the mobility does not depend on the scale, the total current is
$J=\sum_r\alpha_rJ_r$. For the minimal realization, aggregate signed currents
first:
\begin{equation}
 a(x,y)=\frac{[\sum_r\alpha_rJ_r(x,y)]_+}{q(x)}.
 \label{eq:kdd-multiscale-minimal}
\end{equation}
The alternative $\sum_r\alpha_r[J_r(x,y)]_+/q(x)$ has the same signed
marginal current, but can contain unnecessary two-way counterflow and require
a smaller admissible step. It is not the edgewise minimal realization of the
combined field.

\subsubsection{Time-dependent bandwidth is a different analysis}

For a differentiable bandwidth schedule $\tau(t)$, even the exact
instantaneous gradient flow obeys
\begin{equation}
 \frac{d}{dt}\mathcal F_{\tau(t),p}(q_t)
 =-\mathcal I_{\tau(t),K}(q_t\mid p)
    +\dot\tau(t)\,\partial_\tau\mathcal F_{\tau,p}(q_t).
 \label{eq:kdd-annealing}
\end{equation}
Thus fixed-energy monotonicity cannot be asserted without the extra term.
For the heat family, the log-sum inequality implies contraction of KL under
any stochastic channel; applying the additional channel $S_s$ to both laws
gives $\mathcal F_{\tau+s,p}(q)\leq\mathcal F_{\tau,p}(q)$.
Accordingly, decreasing the bandwidth can increase the value of the
comparison objective even without any change in $q$. Start with fixed
single-scale and fixed multiscale experiments before introducing annealing.

\subsection{Numerical specification and efficient implementation}
\label{sec:kdd-numerics}

\subsubsection{A probability bound is not an energy-descent bound}

The global step condition \eqref{eq:kdd-cfl} guarantees a stochastic
transition but not finite-step descent of the energy. For an exact field,
first-order expansion gives
\begin{equation}
 \mathcal F_{\tau,p}(q+\eta v)
 =\mathcal F_{\tau,p}(q)-\eta\mathcal I_{\tau,K}(q\mid p)+O(\eta^2).
 \label{eq:kdd-prob-descent}
\end{equation}
A constructive sufficient bound follows from the Hessian. Let
$a=\min_{x,y}S(x,y)>0$ and
$C_S=\|S\|_{2\to2}^2/a$, where the norm is the ordinary Euclidean matrix
operator norm. Since $rS\geq a\kddone$ for any probability law $r$,
\begin{equation}
 D^2\mathcal F_{\tau,p}(r)[h,h]\leq C_S\|h\|_2^2.
\end{equation}
Along any admissible segment $q+s v$ in the simplex,
\begin{equation}
 \mathcal F_{\tau,p}(q+\eta v)
 \leq\mathcal F_{\tau,p}(q)-\eta\mathcal I_{\tau,K}(q\mid p)
                 +\frac{C_S\eta^2}{2}\|v\|_2^2.
 \label{eq:kdd-sufficient-bound}
\end{equation}
For a desired Armijo fraction $c_A\in(0,1)$, the sufficient additional
condition is
\begin{equation}
 \eta\leq\frac{2(1-c_A)\mathcal I_{\tau,K}(q\mid p)}{C_S\|v\|_2^2}
 \label{eq:kdd-explicit-descent-step}
\end{equation}
when $v\ne0$. This worst-case bound may be overly conservative. In practice,
start with \eqref{eq:kdd-safe-step} and halve $\eta$ until
\begin{equation}
 \mathcal F_{\tau,p}(q+\eta v)
 \leq\mathcal F_{\tau,p}(q)-c_A\eta\mathcal I_{\tau,K}(q\mid p).
 \label{eq:kdd-armijo}
\end{equation}
Keep the field frozen during this search, but recompute the energy of each
candidate law. At an exact interior nonequilibrium point, sufficiently small
steps satisfy the condition. For multiple scales, replace $C_S$ by
$\sum_r\alpha_r\|S_r\|_{2\to2}^2/a_r$. When using a sampled force, neither
this deterministic Armijo guarantee nor descent of a freshly resampled
objective is established. The provided code permits a small declared
roundoff tolerance in the comparison.

\subsubsection{Stable logarithmic-mean weights}

The straightforward expression $L(r)=\operatorname{expm1}(r)/r$ is useful
near ordinary scales but can overflow when $r$ is large and positive.
Computing one symmetric mobility per unordered edge is more robust than
computing the two directional factors independently.

For an edge $\{i,j\}$, let
\begin{equation}
 a=\log q(i)-\log\pi(i),\quad
 b=\log q(j)-\log\pi(j),\quad
 d=|a-b|,
 \qquad
 \phi(d)=\begin{cases}(1-e^{-d})/d,&d>0,\\1,&d=0.\end{cases}
\end{equation}
Then
\begin{align}
 m(e^a,e^b)&=e^{\max(a,b)}\phi(d),
 \label{eq:kdd-stable-mean}\\
 \log w_q(i,j)
  &=\log(\pi(i)K(i,j))+\max(a,b)+\log\phi(d).
 \label{eq:kdd-logweight}
\end{align}
Evaluate $\phi(d)$ using $-\operatorname{expm1}(-d)/d$ away from zero.
Near zero use
\begin{equation}
 \phi(d)=1-\frac d2+\frac{d^2}{6}-\frac{d^3}{24}+\frac{d^4}{120}+O(d^5).
 \label{eq:kdd-phi-series}
\end{equation}
The attached float64 code switches to this polynomial when $d<10^{-4}$.
Forming \eqref{eq:kdd-logweight} before exponentiation avoids an unnecessary
large intermediate relative density. Then compute one signed $J(i,j)$,
set the reverse current to $-J(i,j)$, and derive the two rates by dividing
its positive and negative parts by the corresponding actual masses.
Extremely small $q(x)$ can still produce large rates; the stable formula
cannot remove genuine boundary conditioning.

\paragraph{Potential evaluation and offsets.}
Use $\log q_\tau-\log p_\tau$, rather than forming their quotient before
logging. An additive centering $U\leftarrow U-\sum_xq(x)U(x)$ leaves all
currents unchanged. If working from unnormalized masses, a dense stable
formula for the inner log-ratio is
\begin{align}
 \widetilde\ell(y)
 ={}&\kddLSE_x\bigl(\log\widetilde q(x)+\log S(x,y)\bigr)\nonumber\\
   &-\kddLSE_x\bigl(\log\widetilde p(x)+\log S(x,y)\bigr),
 \label{eq:kdd-logsumexp}
\end{align}
followed by $S\widetilde\ell$. A zero unnormalized mass contributes
$-\infty$ inside its log-sum-exp. This formula preserves the declared
channel and avoids silently adding a probability floor.

\paragraph{No silent repairs.}
Do not silently clamp smoothed masses before taking logarithms, clip rates,
threshold the support of $S$, or renormalize the transported rows. Each
changes an equation used by the proofs. Detect and report invalid or
nonfinite values. Remedies include higher precision, a larger comparison
bandwidth, or the explicitly defined channel floor
\eqref{eq:kdd-channel-floor}; the operator used for the forward and pullback
actions must match. An explicitly positive softmax in real arithmetic may
underflow in floating-point arithmetic, so strict positivity must be checked
numerically as well.

\subsubsection{Sparse teacher multiplication without constructing $P$}

Store one copy of each unordered edge $\{i,j\}$ with an arbitrary consistent
orientation $i\to j$. Let $a_{ij}=[J_{ij}]_+/q_i$ and
$a_{ji}=[-J_{ij}]_+/q_j$, and accumulate the outgoing rates $\lambda_i$.
For a bank of probability rows $R\in\kddR^{B\times N}$, initialize
\begin{equation}
 T_{b,x}\gets R_{b,x}(1-\eta\lambda_x).
 \label{eq:kdd-sparse-teacher-init}
\end{equation}
For each unordered edge, scatter the two incoming contributions
\begin{equation}
 T_{b,j}\mathrel{+}=\eta R_{b,i}a_{ij},
 \qquad
 T_{b,i}\mathrel{+}=\eta R_{b,j}a_{ji}.
 \label{eq:kdd-sparse-teacher-scatter}
\end{equation}
Use the old rows $R$ on both right-hand sides, not partially updated values
of $T$. This computes exactly $T=RP_\eta$ in real arithmetic. No dense
$N\times N$ transport matrix is required. The mobility and rates are built
once from the bank marginal, not separately from each $R_b$.

\subsubsection{FFT specialization for the existing two-dimensional torus}
\label{sec:kdd-torus}

For the manuscript's $n\times n$ periodic grid, $n=32$, take
$\pi=1/n^2$ and $K(x,y)=1/4$ for the four nearest neighbors. Use the same
state flattening for network outputs, grid arrays, and edge indices; the
reference implementation uses $(x_1,x_2)\mapsto nx_1+x_2$.
The Fourier mode indexed by $(k,\ell)$ has
\begin{equation}
 \lambda_{k,\ell}
  =1-\frac12\left(\cos\frac{2\pi k}{n}
                  +\cos\frac{2\pi\ell}{n}\right),
 \qquad 0\leq k,\ell<n.
 \label{eq:kdd-torus-eigenvalue}
\end{equation}
Indeed, shifting a mode by one lattice site multiplies it by the appropriate
complex phase; averaging the four shifts gives the two cosine terms.
Consequently, the heat action is
\begin{equation}
 \mathsf{Heat}_\tau(f)
 =\operatorname{IFFT}_2\left[
         e^{-\tau\lambda_{k,\ell}}\operatorname{FFT}_2(f)\right].
 \label{eq:kdd-fft}
\end{equation}
Because this $K$ and $S_\tau$ are symmetric, the same array routine is used
for mass smoothing and potential pullback:
\begin{equation}
 q_\tau=\mathsf{Heat}_\tau(q),\qquad
 p_\tau=\mathsf{Heat}_\tau(p),\qquad
 U_\tau=\mathsf{Heat}_\tau(\log q_\tau-\log p_\tau).
 \label{eq:kdd-torus-U}
\end{equation}
The inverse FFT is real in exact arithmetic. Discard only the numerical
imaginary part; do not clip negative real values silently. Sparse empirical
laws at a very small bandwidth can produce values below floating-point
resolution even though the mathematical heat kernel is positive.

For the optional channel floor, keep the zero-frequency multiplier equal
to $1$ and multiply every other frequency multiplier by
$1-\varepsilon_s$. At $\tau=0$ with no channel floor and positive $p,q$,
use the identity operator directly to recover the original force without
FFT roundoff.

The factor $1/4$ in $K$ matters: \eqref{eq:kdd-torus-eigenvalue} corresponds
to the normalized random-walk generator $K-I$, not the unnormalized graph
Laplacian. Thus copying a heat-kernel bandwidth from a routine using the latter
requires a time rescaling. The transport step $\eta$ and smoothing time
$\tau$ remain separate parameters.

\paragraph{Cost and caching.}
With $R$ comparison scales and $|\mathcal E_u|$ unordered edges, FFT-based
potential evaluation costs $O(RN\log N)$, edge construction costs
$O(|\mathcal E_u|)$, and exact conditional teachers cost
$O(B|\mathcal E_u|)$. Caching $pS_r$ removes repeated target smoothing when
the target law and channels are fixed. A line search adds candidate energy
evaluations. Dense smoothing instead costs $O(RN^2)$ per potential and stores
$O(RN^2)$ entries if the matrices are retained. A sparse transport graph does
not imply that its heat matrix is sparse. Approximate semigroup routines or
truncated series introduce a further numerical approximation whose
positivity, dual action, and effective operator must be checked.

\paragraph{The global rate maximum at scale.}
On the enumerable torus, $\max_x\lambda_q(x)$ is computable exactly.
A maximum over only sampled states is not a certified global maximum and
does not by itself justify a common stochastic $P_\eta$ on the full space.
A scalable implementation must supply a valid bound or explicitly analyze
a different update rule. This limitation is inherited from the frozen
Euler particle construction, not solved by smoothing.

\subsection{Validation protocol and ablations}
\label{sec:kdd-validation}

The first deliverable should be a new potential routine and tests, not a
simultaneous rewrite of the generator, estimator, and transport. For
comparisons with existing runs, import the actual $p,q_0$, latent bank, and
network initialization from the current experiment code. The supplied
reference demo constructs a problem from the manuscript's printed normalized
parameters; it is not a reproduction of the reported trajectories or a check
against the unavailable original repository.

\subsubsection{Stage I: exact-array algebra}

Use float64 and check the following identities before any training run.
\begin{longtable}{@{}p{0.23\linewidth}p{0.72\linewidth}@{}}
\toprule
Check & Required result \\
\midrule
\endfirsthead
\toprule
Check & Required result \\
\midrule
\endhead
Channel structure & $S\kddone=\kddone$, $\pi S=\pi$, detailed balance, and
positive entries for the declared finite positive-scale channel. \\[3pt]
Dual orientation & $(hS)f=h(Sf)$ on a reversible chain with nonuniform $\pi$
and nonsymmetric $S$. A torus-only check is insufficient. \\[3pt]
First variation & For zero-sum $h$, compare
$[\mathcal F(q+\epsilon h)-\mathcal F(q-\epsilon h)]/(2\epsilon)$ to
$\sum_xh(x)U(x)$. \\[3pt]
Hessian & Compare the directional derivative of $U$ to
$\sum_y(hS)(y)^2/(qS)(y)$; the quadratic form is positive for $h\ne0$. \\[3pt]
Current and gauge & Reverse currents are negatives; adding a constant to $U$
changes no current; $\sum_xv(x)=0$ and $\sum_xq(x)\Delta(x)=0$. \\[3pt]
Dissipation & $\sum_xU(x)v(x)=-\mathcal I$ and the finite-difference energy
derivative approaches this value. \\[3pt]
Traffic realization & $q(x)a(x,y)-q(y)a(y,x)=J(x,y)$ and minimal total
traffic equals $|J(x,y)|$. \\[3pt]
Probability Euler & $qP_\eta=q+\eta v$ to floating-point tolerance;
$P_\eta$ is stochastic for a valid common step. \\[3pt]
Teacher linearity & For the same frozen $P_\eta$,
$B^{-1}\sum_bR_bP_\eta=(B^{-1}\sum_bR_b)P_\eta$. \\[3pt]
Chart consistency & The discrepancy between $q_{g+\eta\Delta}$ and
$qP_\eta$ scales as $O(\eta^2)$ before roundoff dominates. \\[3pt]
Limiting cases & Exact equality $q=p$ gives zero potential difference and
zero rates; $\tau=0$ with positive laws recovers the original method. \\[3pt]
Torus implementation & On a smaller torus, FFT and a dense matrix
exponential give the same forward and pullback actions. \\[3pt]
Spectral scaling & Near $p=\pi$, a single mode has derivative coefficient
$-\lambda e^{-2\tau\lambda}$, or the multiscale counterpart. \\[3pt]
Sparse comparison & Empirical comparison laws with zeros produce finite
smoothed potentials, but using a sparse law as the transported $q$ is rejected. \\
\bottomrule
\end{longtable}
A central finite difference has $O(\epsilon^2)$ truncation error for a
smooth energy, until floating-point cancellation dominates. Choose
perturbations small enough that $q\pm\epsilon h$ stay positive, and do not
judge an order test using residuals at the numerical floor. The reference
suite implements twenty controlled tests spanning these checks, including
multiscale and channel-floor cases.

\subsubsection{Stage II: exact flow before estimation}

Keep all distributional quantities exact. Compare the original flow
($\tau=0$), several fixed positive bandwidths, and a fixed multiscale energy.
A starting sweep in the time units of \eqref{eq:kdd-heat} is
$\tau\in\{0.25,1,4,16\}$, but these are experimental suggestions, not
optimized values. The reference smoke test uses equal weights on
$\tau\in\{0.5,2,8\}$. Retain the existing step-size cap as a starting
configuration, but enforce the new field's rate bound and optionally use
backtracking rather than assuming the old admissible step remains valid.

Log the smoothed energy, its predicted dissipation, true total variation to
$p$, true unsmoothed KL when finite, minimum model mass, maximum exit rate,
minimum stay probability, current antisymmetry residual, and total mass
error. Compare trajectories at the accumulated accepted flow time
$t_k=\sum_{j<k}\eta_j$, not just at equal iteration counts. Report computational
cost separately: equal flow time is not equal wall-clock work.

\subsubsection{Stage III: isolate statistical regularization}

First sample only the target in \eqref{eq:kdd-target-only-estimation}, while
retaining exact model smoothing and exact mobility. Then sample the model
comparison as well. Only after these checks should outer Monte Carlo or a
learned ratio estimator be added. For a fixed target dataset, hold it fixed
across compared methods and distinguish its empirical energy from the
population diagnostics available in the synthetic test.

The principal statistic is the edgewise potential error
$\|\widehat U-U\|_{q,K}$, measured at a common $q$. Compare it to the true
force size $\|U\|_{q,K}$. Also record the local teacher-law discrepancy in
\eqref{eq:kdd-step-error}. This tests whether smoothing reduces force error
enough to compensate for the attenuated population dynamics. A small
smoothed energy alone is insufficient evidence, since increasing the
bandwidth makes all distributions look closer.

Useful controls are target-only smoothing with energy
$\kddKL(q\|pS)$ and the direct smoothed-log-ratio force
$\widetilde U=\log(qS/pS)$. Label these as different methods. The first
has population target $pS$; the second is not the exact gradient of the
smoothed-KL energy derived here. Any pseudocount baseline for an unsmoothed
empirical log-ratio must state the pseudocount and the resulting altered law.

\subsubsection{Stage IV: neural amortization}

Keep the generator architecture, initialization, latent prior/bank, and
inner fitting budget fixed while replacing the transport teacher routine.
Construct a conditional oracle that uses the same channels and exact teacher
multiplication but no neural fitting. Report local fitting error,
marginal fitting error, and accumulated neural--oracle discrepancy separately.
Held-out latent teachers must use the training marginal's frozen transition,
not a newly constructed held-out transition. When introducing a finite
latent-batch approximation, state whether that batch defines both the
marginal used to build the field and the conditionals being fitted.

Do not infer improved real-data performance from passing algebraic tests or
from the reference smoke test. Those checks validate the finite-state
specification and its implementation only.

\subsection{Optional alternative: a kernel-MMD discrepancy}
\label{sec:kdd-mmd}

The primary implementation above retains KL, evaluated after smoothing.
A separate option is useful when the potential should be a difference of
unbiased kernel sample averages without logarithms. This option changes the
energy, not the transport geometry, and is not part of the default update.

Using the symmetric kernel \eqref{eq:kdd-kappa}, define
\begin{align}
 \mathcal E_{\tau,p}(q)
 &=\frac12\sum_{x,y}(q-p)(x)\kappa_\tau(x,y)(q-p)(y)\nonumber\\
 &=\frac12\langle\rho_q-\rho_p,
                    S_\tau(\rho_q-\rho_p)\rangle_\pi.
 \label{eq:kdd-mmd-energy}
\end{align}
This is one half of the squared maximum mean discrepancy (MMD) for
$\kappa_\tau$. Symmetry gives the first variation
\begin{align}
 U^{\rm MMD}_{\tau,p,q}(x)
   &=\sum_y\kappa_\tau(x,y)(q-p)(y)\nonumber\\
   &=\kddE_{Y\sim q}[\kappa_\tau(x,Y)]
       -\kddE_{Y\sim p}[\kappa_\tau(x,Y)].
 \label{eq:kdd-mmd-U}
\end{align}
Proposition~\ref{prop:kdd-heat} gives strict convexity and unique minimizer~$p$.
Substituting this potential into \eqref{eq:kdd-current} gives
\begin{equation}
 \frac{d}{dt}\mathcal E_{\tau,p}(q_t)
   =-\|U^{\rm MMD}_{\tau,p,q_t}\|_{q_t,K}^2\leq0.
\end{equation}
Minimal particles and frozen conditional teachers follow by the same
current identities. A finite-sample average estimates
\eqref{eq:kdd-mmd-U} without logarithmic ratio bias, but its positive-part
jump rates need not be unbiased. The dependence on the unsmoothed mobility,
the interior-law requirement, and the need for an admissible step are all
unchanged. This method descends MMD, not KL. Validate it as a separate
ablation rather than mixing its force with the primary formula without
specifying a combined energy.

\subsection{Handoff and reference-code interface}
\label{sec:kdd-handoff}

The accompanying \texttt{reference\_implementation.py} implements the finite-state
specification in float64 NumPy/SciPy. It is a standalone reference, not a patch
to an existing training repository. Its principal interfaces are:

\begingroup\small
\begin{longtable}{@{}p{0.36\linewidth}p{0.59\linewidth}@{}}
\toprule
Interface & Meaning \\
\midrule
\endfirsthead
\toprule
Interface & Meaning \\
\midrule
\endhead
\texttt{DenseHeatSmoother} & Dense general reversible channel, with distinct
mass-push and function-pull actions. \\[2pt]
\texttt{TorusHeatSmoother} & FFT channel on the periodic grid, with an optional
explicit channel floor. \\[2pt]
\texttt{SmoothedKL.evaluate(q)} & Energy and exact potential, including outer
smoothing; supports fixed multiscale weights. \\[2pt]
\texttt{EdgeGeometry} & Unordered edges and conductances $\pi(i)K(i,j)$. \\[2pt]
\texttt{build\_field(q,U,geometry)} & Stable weights, currents, minimal rates,
exit rates, probability/logit drifts, and dissipation; requires $q>0$. \\[2pt]
\texttt{FrozenField.advance(R,eta)} & Apply one common frozen Euler transition
to a probability row or a conditional bank. \\[2pt]
\texttt{armijo\_step} & Global stochasticity bound and exact-energy
backtracking; no sampled-force descent guarantee. \\[2pt]
\texttt{empirical\_law} & Histogram for comparison only, not for the
transported positive marginal. \\
\bottomrule
\end{longtable}
\endgroup

For the current enumerable experiment, the essential insertion is:
\begin{lstlisting}[style=kddpython]
# R: [number_of_latents, number_of_states]; objective caches the target.
q = R.mean(axis=0)                   # actual, unsmoothed marginal
value, U = objective.evaluate(q)     # forward AND outer smoothing
field = build_field(q, U, geometry)  # mobility still comes from q
eta = field.safe_step(eta_cap=0.8, safety=0.9)
T = field.advance(R, eta)            # same transition for all latents
# Detach T; fit the generator by conditional cross-entropy.
\end{lstlisting}
The constants are starting settings, not energy-descent guarantees; use
\texttt{armijo\_step} when needed. Neural fitting, scalable marginal-ratio
estimation, a global rate bound on nonenumerable spaces, and the optional
MMD method are not included in the reference code.

\paragraph{Acceptance criterion.}
Before neural ablations, require the nonuniform-orientation, first-variation,
dissipation, probability-Euler, teacher-linearity, zero-bandwidth, and FFT
tests to pass. Then measure whether sample-based comparison improves the
usable training signal while preserving the one-step inference interface.
e
